# Supplementary material for: Significance tests of feature relevance for a black-box learner
Source: arXiv:2103.04985 source file (2022-06-21)
Supplement: Supplementary file 1 [file TNNLS-2021-P-17585_sppul.tex]

\documentclass[journal]{IEEEtran}
%
% If IEEEtran.cls has not been installed into the LaTeX system files,
% manually specify the path to it like:
% \documentclass[journal]{../sty/IEEEtran}

\usepackage{hhline,bm,xcolor,amsmath}
\usepackage{amssymb}
\usepackage{graphicx,multirow,booktabs,subfigure,comment}
\usepackage[linesnumbered,ruled]{algorithm2e}
\usepackage{caption}
% \usepackage{hhline,bm,amssymb,epsfig,amsmath,array,amsthm,xcolor}

% Definitions of handy macros can go here

\def\argmin{\mathop{\rm argmin}}

\def\Cov{\mathop{\rm Cov}}
\def\Var{\mathop{\rm Var}}
\def\sign{\mathop{\rm Sign}}

\usepackage{mathtools}

\makeatletter
\newcommand*{\rom}[1]{\expandafter\@slowromancap\romannumeral #1@}
\makeatother
\newcommand*{\EOP}{\hfill\ensuremath{\square}}%

% Some very useful LaTeX packages include:
% (uncomment the ones you want to load)
\newtheorem{theorem}{Theorem}[section]
\newtheorem{lemma}[theorem]{Lemma}

\numberwithin{equation}{section}
\numberwithin{table}{section}
\numberwithin{figure}{section}
% *** MISC UTILITY PACKAGES ***
%
%\usepackage{ifpdf}
% Heiko Oberdiek's ifpdf.sty is very useful if you need conditional
% compilation based on whether the output is pdf or dvi.
% usage:
% \ifpdf
%   % pdf code
% \else
%   % dvi code
% \fi
% The latest version of ifpdf.sty can be obtained from:
% http://www.ctan.org/pkg/ifpdf
% Also, note that IEEEtran.cls V1.7 and later provides a builtin
% \ifCLASSINFOpdf conditional that works the same way.
% When switching from latex to pdflatex and vice-versa, the compiler may
% have to be run twice to clear warning/error messages.

% *** CITATION PACKAGES ***
%
%\usepackage{cite}
% cite.sty was written by Donald Arseneau
% V1.6 and later of IEEEtran pre-defines the format of the cite.sty package
% \cite{} output to follow that of the IEEE. Loading the cite package will
% result in citation numbers being automatically sorted and properly
% "compressed/ranged". e.g., [1], [9], [2], [7], [5], [6] without using
% cite.sty will become [1], [2], [5]--[7], [9] using cite.sty. cite.sty's
% \cite will automatically add leading space, if needed. Use cite.sty's
% noadjust option (cite.sty V3.8 and later) if you want to turn this off
% such as if a citation ever needs to be enclosed in parenthesis.
% cite.sty is already installed on most LaTeX systems. Be sure and use
% version 5.0 (2009-03-20) and later if using hyperref.sty.
% The latest version can be obtained at:
% http://www.ctan.org/pkg/cite
% The documentation is contained in the cite.sty file itself.

% *** GRAPHICS RELATED PACKAGES ***
%
\ifCLASSINFOpdf
  % \usepackage[pdftex]{graphicx}
  % declare the path(s) where your graphic files are
  % \graphicspath{{../pdf/}{../jpeg/}}
  % and their extensions so you won't have to specify these with
  % every instance of \includegraphics
  % \DeclareGraphicsExtensions{.pdf,.jpeg,.png}
\else
  % or other class option (dvipsone, dvipdf, if not using dvips). graphicx
  % will default to the driver specified in the system graphics.cfg if no
  % driver is specified.
  % \usepackage[dvips]{graphicx}
  % declare the path(s) where your graphic files are
  % \graphicspath{{../eps/}}
  % and their extensions so you won't have to specify these with
  % every instance of \includegraphics
  % \DeclareGraphicsExtensions{.eps}
\fi

\usepackage{lipsum}
\usepackage{fancyhdr}

\pagestyle{fancy}
\fancyhf{}
\cfoot{\thepage}

\fancypagestyle{sec}{\lhead{\tmpx}}

\fancypagestyle{arXiv}
{
   \fancyhf{}
   
   \chead{\textcolor{gray}{This paper has been accepted for publication at the \\ IEEE Transactions on Neural Networks and Learning Systems,  2022}}
   
   \cfoot{\vspace{-6mm} \fontsize{=6pt}{10pt}\selectfont  \textcolor{gray}{© 2022 IEEE. Personal use of this material is permitted. Permission from IEEE must be obtained for all other uses, in any current or future media, including reprinting/republishing this material for advertising or promotional purposes, creating new collective works, for resale or redistribution to servers or lists, or reuse of any copyrighted component of this work in other works}\\\fontsize{=10pt}{12pt}\selectfont\thepage}
   
}

% *** PDF, URL AND HYPERLINK PACKAGES ***
%
%\usepackage{url}
% url.sty was written by Donald Arseneau. It provides better support for
% handling and breaking URLs. url.sty is already installed on most LaTeX
% systems. The latest version and documentation can be obtained at:
% http://www.ctan.org/pkg/url
% Basically, \url{my_url_here}.

% *** Do not adjust lengths that control margins, column widths, etc. ***
% *** Do not use packages that alter fonts (such as pslatex).         ***
% There should be no need to do such things with IEEEtran.cls V1.6 and later.
% (Unless specifically asked to do so by the journal or conference you plan
% to submit to, of course. )

% correct bad hyphenation here
\hyphenation{op-tical net-works semi-conduc-tor}

\begin{document}
%
% paper title
% Titles are generally capitalized except for words such as a, an, and, as,
% at, but, by, for, in, nor, of, on, or, the, to and up, which are usually
% not capitalized unless they are the first or last word of the title.
% Linebreaks \\ can be used within to get better formatting as desired.
% Do not put math or special symbols in the title.
\title{Supplementary Materials for ``Significance Tests of Feature Relevance for a Black-Box Learner''}
%
%
% author names and IEEE memberships
% note positions of commas and nonbreaking spaces ( ~ ) LaTeX will not break
% a structure at a ~ so this keeps an author's name from being broken across
% two lines.
% use \thanks{} to gain access to the first footnote area
% a separate \thanks must be used for each paragraph as LaTeX2e's \thanks
% was not built to handle multiple paragraphs
%

\author{
  Ben Dai,
  Xiaotong Shen,
  and Wei Pan
  \thanks{Ben Dai is with the Department of Statistics, The Chinese University of Hong Kong, Hong Kong SAR (email: bendai@cuhk.edu.hk).} 
  
  \thanks{Xiaotong Shen is with the School of Statistics, University of Minnesota, MN, 55455 USA (email: xshen@umn.edu).}

  \thanks{Wei Pan is with the Division of Biostatistics, University of Minnesota, MN, 55455 USA. (email: panxx014@umn.edu).}
}

\maketitle

% For peer review papers, you can put extra information on the cover
% page as needed:
% \ifCLASSOPTIONpeerreview
% \begin{center} \bfseries EDICS Category: 3-BBND \end{center}
% \fi
%
% For peerreview papers, this IEEEtran command inserts a page break and
% creates the second title. It will be ignored for other modes.
\IEEEpeerreviewmaketitle

\appendices
\section{Two-split test}
\thispagestyle{arXiv}

To treat the high \textit{bias-sd-ratio} issue as described in Section 2, we propose an alternative of the one-split test by further splitting an inference sample into two equal subsamples yet the perturbation is not required. For simplicity, we assume $m$ is an even number.

\subsection{Two-split test}
Given $(\widehat{f}_n,\widehat{g}_n)$, we evaluate them based on these two independent subsamples to yield our two-split test statistic:
\begin{align}
\label{eqn:TS_statistic}
& \Lambda^{(2)}_n = \frac{ \sum_{j=1}^{m/2} \Delta^{(2)}_{n,j}}{ \sqrt{\frac{m}{2}} \widehat{\sigma}^{(2)}_n}, \\
& \Delta^{(2)}_{n,j} = l(\widehat{f}_n(\bm{X}_{n+j}), \bm{Y}_{n+j}) - l(\widehat{g}_n(\bm{Z}_{n+m+j}), \bm{Y}_{n+m+j}), \nonumber
\end{align}
where $\widehat{\sigma}^{(2)}_n$ is the sample standard deviation of $\{ \Delta^{(2)}_{n,j} \}_{j=1}^{m/2}$ given $\widehat{f}_n$ and $\widehat{g}_n$. In this fashion, perturbation 
is no longer required.

Similarly, the two-split test proceeds as the one-split test except that its $p$-value is computed as $P^{(2)}=\Phi(\Lambda^{(2)}_n)$ based on Theorem \ref{thm:type1}.

To derive the asymptotic null distribution of $\Lambda^{(2)}_n$, we make the parallel assumptions B$'$ and C$'$.

\noindent \textbf{Assumption B$'$} (Lyapounov condition for $\Lambda^{(2)}_n$). Assume that
$$
 m^{-\mu} \mathbb{E} \big( | \Delta^{(2)}_{n,1} |^{2(1+\mu)} \big| \mathcal{E}_n \big) \stackrel{p}{\longrightarrow} 0, \quad \text{as } n \rightarrow \infty
$$
for some constant $\mu > 0$,
where $\Delta^{(2)}_{n,1}$ is defined in \eqref{eqn:TS_statistic} and $
 \stackrel{p}{\longrightarrow}$ denotes convergence in probability. 

\noindent \textbf{Assumption C$'$} (Variation) Assume that $\Var( \Delta^{(2)}_{n,1} | \mathcal{E}_n ) \stackrel{p}{\longrightarrow} (\sigma^{(2)})^2$ as 
$n \to \infty$.

Under some mild assumptions, $(\sigma^{(2)})^2 = \Var \big( l(f^*(\bm{X}), \bm{Y}) \big) + \Var \big( l(g^*(\bm{Z}(\bm{X})), \bm{Y}) \big) > 0$, c.f., Lemma \ref{lem:example}.

\begin{theorem}[Asymptotic null distribution]
\label{thm:type1} 
In addition to Assumptions A, B$'$, and C$'$, if $m = o(n^{2\gamma})$, then under $H_0$,
\begin{equation}
\label{eqn:asy_dis2}
\Lambda^{(2)}_n \stackrel{d}{\longrightarrow} N(0,1), \quad \text{as} \quad n \to \infty.
\end{equation}
\end{theorem}
Furthermore, the $p$-value $\bar{P}^{(2)}$ for the combined two-split test can be defined exactly as in Section 2.3.

\begin{theorem}[Type \rom{1} error for the combined two-split test]
\label{thm:TS_subsamples_type1} 
Suppose that Assumption A and $B'$-$C'$ are satisfied for the two-split test \eqref{eqn:TS_statistic}, if $m = o(n^{2\gamma})$, then under $H_0$, for any $0<\alpha<1$ and any $U \geq 2$, 
\begin{equation*}
% \label{eqn:asy_disc}
\lim_{n \to \infty} \mathbb{P} \big(\bar{P}^{(2)} \leq \alpha | H_0 \big) \leq \alpha,
\end{equation*}
where $\bar{P}^{(2)}$ is defined as the $q$-order test or the Hommel's test based on ($P_1^{(2)}, \cdots, P^{(2)}_U$).
\end{theorem}

\subsection{Type \rom{2} error for two-split tests}
This section performs Type \rom{2} error analysis of the two-split test in \eqref{eqn:TS_statistic}. Consider an alternative hypothesis $H_a: R(f^*) - R_\mathcal{S}(g^*) = - m^{-1/2} \delta < 0$ for $\delta>0$. The Type \rom{2} error of the two-split test in \eqref{eqn:TS_statistic} and its combined tests can be written as 
\begin{align*}
\beta_n^{(2)}(\delta) = \mathbb{P} (P^{(2)} \geq \alpha | H_a ), \quad  \bar{\beta}_n^{(2)}(\delta) = \mathbb{P} ( \bar{P}^{(2)} \geq \alpha | H_a ),
\end{align*}
where $\mathbb{P}(\cdot|H_a)$ denotes the probability under $H_a$ and $\alpha > 0$ is the nominal level.

Theorems \ref{thm:TS_power} and \ref{thm:TS_cp_power} suggest that the Type \rom{2} error of the two-split test and its combined test tend to zero as $\delta \rightarrow \infty$.

\begin{theorem}[Limiting Type \rom{2} error of the two-split test]
\label{thm:TS_power}
Under Assumption A, $B'$ and $C'$, if $m = o(n^{2\gamma})$, then we have
\begin{align}
& \lim_{n \to \infty} \sup \beta_n^{(2)}(\delta)= \Phi\Big( z_\alpha -\frac{\delta}{\sqrt{2}\sigma^{(2)}} \Big), \nonumber \\
& \lim_{\delta \to \infty} \lim_{n \to \infty} \sup \beta_n^{(2)}(\delta)= 0,
\end{align}
where $z_\alpha = \Phi^{-1}(1-\alpha)$ is the $100(1-\alpha)$th percentile of the standard normal distribution.
\end{theorem}

\begin{theorem}[Limiting Type \rom{2} error of the combined two-split test]
\label{thm:TS_cp_power}
Under Assumption A, B$'$ and C$'$, $m = o(n^{2\gamma})$, then for $\bar{P}^{(2)}$ defined as the $q$-order combined test, we have
\begin{align*}
&  \lim_{n \to \infty} \sup \bar{\beta}_n^{(2)}(\delta) \leq \min\Big(\frac{U}{\alpha q} \Gamma,1\Big), \\
& \lim_{\delta \to \infty} \lim_{n \to \infty} \sup \bar{\beta}_n^{(2)}(\delta)= 0, 
\end{align*}
and for $\bar{P}^{(2)}$ defined as the Hommel combined test, we have
\begin{align*}
&  \lim_{n \to \infty} \sup \bar{\beta}_n^{(2)}(\delta) \leq \min  \Big\{ \frac{C_U U}{\alpha q} \Gamma,1; q =1, \cdots, U\Big\}, \\ 
& \lim_{\delta \to \infty} \lim_{n \to \infty} \sup \bar{\beta}_n^{(2)}(\delta)= 1, 
\end{align*}
where $\Gamma =  \Phi\big(-\frac{\delta}{2 \sigma^{(l)}} \big) + \sqrt{\frac{q - 1}{U- q +1}} \Big( \Phi\big(\frac{\delta}{ 2 \sigma^{(l)}} \big) - \Phi^{2}\big(\frac{\delta}{2 \sigma} \big) - 2T(- \frac{\delta}{2 \sigma^{(l)}}, \frac{\sqrt{3}}{3}) \Big)^{1/2}$, and
$T(h,a)=(2 \pi)^{-1} \int_{0}^a
\frac{\exp(-h^2(1+x^2)/2)}{x^2+1} dx$ is Owen's $T$ function \cite{owen1956tables}.
%$C_U = \sum_{u=1}^U u^{-1}$.
\end{theorem}

\subsection{Data-adaptive sample splitting for the two-split test}
This section develops a computing scheme to determine the sample splitting ratio or $\zeta$ to achieve our objective of controlling Type \rom{1} error in a finite-sample situation. 

% Our strategy of adaptive sample splitting and tuning is to generate  permutation samples under $H_0$ and estimate Type \rom{1} error based on permuted inference samples while fitting $\widehat{f}_n$ and $\widehat{g}_n$ only once on an estimation sample to reduce the computational cost. 
% To generate a permuted sample, we permute the hypothesized features of the dataset, that is, permuting $\{ \bm{X}_i, Y_i \}_{i=1}^N = \{\bm{X}_{i,\mathcal{S}}, \bm{X}_{i, \comp{\mathcal{S}}}, Y_i\}_{i=1}^N$ to $\{ \tilde{\bm X}_i,\tilde{Y}_i \}_{i=1}^N =\{ \bm{X}_{\pi(i),\mathcal{S}}, \bm{X}_{i, \comp{\mathcal{S}} }, Y_i\}_{i=1}^N$, where $\pi$ is a permutation. Thus, the hypothesized features for this permuted sample are irrelevant to the prediction of the outcome. 

% Given a ratio value $\zeta$, we first split the dataset as an estimation sample $\{\bm{X}_i, Y_i\}_{i=1}^n$ and an inference sample $\{\bm{X}_i, Y_i\}_{i=n+1}^N$. Then, we permute the estimation sample to generate a permuted estimation sample $\{\tilde{\bm{X}}_i, \tilde{Y}_i \}_{i=1}^n$, which is used for fitting $\widehat{f}_n$ and $\widehat{g}_n$. 
% Then we permute the inference sample $T$ times, denoted by $\pi^{(t)}$; $t=1, \cdots, T$, to generate $T$ permuted samples $(\tilde{\bm X}^{(t)}_i, \tilde{Y}^{(t)}_i)_{i=n+1}^N$; $t=1,\cdots,T$, to estimate Type \rom{1} error.

 Type \rom{1} error of the two-split test is $\text{Err}^{(2)}(\rho, \zeta)= \mathbb{P}(\Lambda_n^{(2)} \leq z_{\alpha} | H_0 )$, which is a function of splitting ratio $\zeta$:
\begin{align}
\label{eqn:TS_type1_err}
\widehat{\text{Err}^{(2)}}(\zeta) = T^{-1} \sum_{t=1}^T \mathbb{I}\big(
\Lambda^{(2,t)}_n \leq z_{\alpha} \big),
\end{align}
where $\Lambda^{(l,t)}_n$; $l=1,2$, computed based on the permuted estimation sample $\{\tilde{\bm{X}}^{(t)}_j, \tilde{Y}^{(t)}_j\}_{j=1}^n$ and the permuted inference sample $\{\tilde{\bm{X}}^{(t)}_j, \tilde{Y}^{(t)}_j\}_{i=n+1}^{N}$; $t = 1, \cdots, T$.

Moreover, data-adaptive is also applicable to the two-split test:
\begin{equation}
\widehat{\zeta} = \min \{ \zeta \in \bm{\zeta} : \widehat{\text{Err}^{(2)}}(\zeta) \leq \alpha\},
\label{eqn:TS_split}
\end{equation}
where $\widehat{\text{Err}^{(2)}}(\zeta)$ is computed via \eqref{eqn:TS_type1_err}.
Furthermore, $\zeta$ for the combined tests are estimated by replacing $P^{(2)}$ by $\bar{P}^{(2)}$ based on permuted sample. The computational scheme of the proposed two-split tests is summarized in Algorithm \ref{algo:TS}.

\begin{algorithm}
    \SetKwInOut{Input}{Input}
    \SetKwInOut{Output}{Output}
    \Input{{Data: $(\bm{x}_i, \bm{y}_i)_{i=1}^N$; Set of hypothesized features: $\mathcal{S}$; Number of splitting: $U$}}
    \Output{$p$-value for the test in Section 2.}
    Estimate $\widehat{\zeta}$ from \eqref{eqn:TS_split} \;
    \For{$u = 1, \cdots, U$}
      {
      Shuffle data\;
      Split data into an estimation sample and an inference sample, where $m = \hat{\zeta}N$ and $n = N - m$\;
      Generate dual samples via (1) for estimation/inference subsets\;
      Compute $\Lambda^{(2)}_u$ from \eqref{eqn:TS_statistic}\;
      Compute $p$-value $P^{(2)}_{u} = \Phi(\Lambda^{(2)}_u)$
      } 
  \uIf(\tcp*[f]{combined two-split test}){$U > 1$}
   { Compute the combined $p$-value $\bar{P}^{(2)}$ via Section 2.3\;
   \Return{$p$-value $\bar{P}^{(2)}$}
   }
  \Else(\tcp*[f]{non-combined two-split test}){
  \Return{$p$-value $P^{(2)}_1$}}
    \caption{Two-split test for feature relevance to prediction.}
    \label{algo:TS}
\end{algorithm}

% you can choose not to have a title for an appendix
% if you want by leaving the argument blank
\section{Additional numerical examples}

\subsection{Numerical results for simulated examples}
The numerical results for Examples 3-6 are indicated in Tables \ref{tab:sim_nets}, \ref{tab:sim_K}, \ref{tab:sim_cor}, and \ref{tab:sim_cp}, respectively.

\begin{table*}[!ht]\centering
  \scalebox{1.0}{
  \begin{tabular}{@{}cccccccccccccccc@{}} \toprule
  % $L=3, d=128, \tau = 2, \rho=.25$ \\
  \phantom{a} & Test & \phantom{a} & $L$ & \phantom{a} & \#Parameters & \phantom{a} & width $\varpi$ & \phantom{a}& Type \rom{1} error & \phantom{a}& \multicolumn{1}{c}{Power (1 - Type II error)} & \phantom{a} & \multicolumn{1}{c}{Time (Second)} &  \\
  \midrule
  & One-split && 2 && 3232 && 32 && 0.050 && (0.26, 0.82, 0.84) && 36.91(0.21) \\
  &  &&  && 6464 && 64 && 0.041 && (0.27, 0.84, 0.89) && 35.48(0.17) \\
  &  &&  && 12928 && 128 && 0.048 && (0.22, 0.90, 0.91) && 35.31(0.18) \\
  \cmidrule{4-15}
  & && 3 && 4256 && 32 && 0.054 && (0.66, 1.00, 1.00) && 39.44(0.29) \\
  & &&   && 10560 && 64 && 0.051 && (0.65, 1.00, 1.00) && 38.41(0.24) \\
  & &&   && 29312 && 128 && 0.050 && (0.61, 0.99, 1.00) && 41.24(0.29) \\
  \cmidrule{4-15}
  & && 4 && 5280 && 32 && 0.066 && (0.98, 1.00, 1.00) && 42.27(0.22) \\
  & &&   && 18752 && 64 && 0.048 && (1.00, 1.00, 1.00) && 41.81(0.30) \\
  & &&   && 62080 && 128 && 0.054 && (0.99, 1.00, 1.00) && 43.12(0.43) \\
  \midrule
  & Two-split && 2 && 3232 && 32 && 0.050 && (0.03, 0.16, 0.13) && 35.76(0.20) \\
  &  &&  && 6464 && 64 && 0.050 && (0.04, 0.11, 0.13) && 35.28(0.30) \\
  &  &&  && 12928 && 128 && 0.055 && (0.05, 0.14, 0.16) && 33.65(0.16) \\
  \cmidrule{4-15}
  & && 3 && 4256  && 32 && 0.044 && (0.19, 0.63, 0.63) && 37.19(0.20) \\
  & &&   && 10560 && 64 && 0.035 && (0.16, 0.47, 0.62) && 35.82(0.20) \\
  & &&   && 29312 && 128 && 0.035 && (0.18, 0.51, 0.58) && 37.02(0.16) \\
  \cmidrule{4-15}
  & && 4 && 5280  && 32  && 0.044 && (0.54, 1.00, 1.00) && 43.54(0.34) \\
  & &&   && 18752 && 64  && 0.041 && (0.54, 1.00, 1.00) && 40.28(0.26) \\
  & &&   && 62080 && 128 && 0.045 && (0.54, 1.00, 1.00) && 47.07(0.31) \\
  \midrule
  & Comb. one-split && 2 && 3232 && 32 && 0.046 && (0.39, 0.98, 0.94) && 61.99(0.17) \\
  & && && 6464 && 64 && 0.022 && (0.22, 0.97, 0.97) && 61.40(0.16) \\
  & && && 12928 && 128 && 0.020 && (0.40, 1.00, 1.00) && 60.42(0.45)  \\
  \cmidrule{4-15}
  &  && 3 && 4256  && 32  && 0.049 && (0.80, 1.00, 1.00) && 63.71(0.21) \\
  &  &&   && 10560 && 64  && 0.032 && (0.79, 1.00, 1.00) && 65.23(0.14) \\
  &  &&   && 29312 && 128 && 0.046 && (0.86, 1.00, 1.00) && 68.28(0.26) \\
  \cmidrule{4-15}
  &  && 4 && 5280 && 32 && 0.054 && (1.00, 1.00, 1.00) && 145.38(0.73) \\
  &  &&   && 18752 && 64 && 0.032 && (1.00, 1.00, 1.00) && 112.77(1.15) \\
  &  &&   && 62080 && 128 && 0.032 && (1.00, 1.00, 1.00) && 127.07(0.79) \\ 
  \midrule
  & Comb. two-split && 2 && 3232 && 32 && 0.022 && (0.00, 0.08, 0.11) && 30.32(0.12) \\
  &  && && 18752 && 64 && 0.015 && (0.06, 0.09, 0.15) && 31.73(0.10) \\
  &  && && 12928 && 128 && 0.017 && (0.04, 0.13, 0.08) && 33.44(0.12) \\
  \cmidrule{4-15}
  &  && 3 && 4256 && 32 && 0.011 && (0.08, 0.75, 0.76) && 41.46(0.34) \\
  &  &&   && 10560 && 64 && 0.007 && (0.08, 0.66, 0.67) && 34.27(0.27) \\
  &  &&   && 29312 && 128 && 0.030 && (0.10, 0.70, 0.65) && 76.28(0.54) \\
  \cmidrule{4-15}
  &  && 4 && 4256 && 32 && 0.013 &&  (0.65, 1.00, 1.00) && 48.99(0.61) \\
  &  &&   && 18752 && 64 && 0.025 &&  (0.65, 1.00, 1.00) && 39.13(0.07) \\
  &  &&   && 62080 && 128 && 0.014 && (0.69, 1.00, 1.00) && 49.05(0.15) \\
  \bottomrule
  \end{tabular}}
  \caption{Type \rom{1} errors and powers of the one-split and two-split tests and their combined tests in Example 3 at a nominal level $\alpha = 0.05$.}
  \label{tab:sim_nets}
  \end{table*}

\begin{table}[!ht]
  \caption{Type \rom{1} errors and powers of the one-split and two-split tests and their combined tests in Example 4 at a nominal level $\alpha = 0.05$. The data-adaptive tuning scheme is applied.}
  \centering
  \scalebox{.87}{
  \begin{tabular}{@{}cccccccccccccc@{}} \toprule
  & Test & \phantom{a} & $|\mathcal{S}_0|$ & \phantom{a}& Type \rom{1} error & \phantom{a}& Power(1 - Type II error) \\
  \midrule
  & One-split && 3 && 0.047 && (0.28, 0.95, 0.96) \\
  & && 5  && 0.050 && (0.61, 0.99, 1.00) \\
  & && 10 && 0.037 && (1.00, 1.00, 1.00) \\
  \midrule
  & Two-split && 3 && 0.052 && (0.09, 0.19, 0.31) \\
  & && 5  && 0.035 && (0.18, 0.51, 0.58) \\
  & && 10 && 0.042 && (0.59, 0.95, 0.98) \\
  \midrule
  & Comb. one-split && 3 && 0.035 && (0.24, 1.00, 1.00)  \\
  & && 5  && 0.046 && (0.86, 1.00, 1.00) \\
  & && 10 && 0.019 && (1.00, 1.00, 1.00) \\
  \midrule
  & Comb. two-split && 3 &&  0.020 && (0.05, 0.20, 0.19) \\
  & && 5  && 0.030 && (0.10, 0.70, 0.65) \\
  & && 10 && 0.013 && (0.72, 1.00, 1.00) \\
  \bottomrule
  \end{tabular}}
  \label{tab:sim_K}
  \end{table}
  
  \begin{table}[!ht]
    \caption{Empirical Type \rom{1} errors and powers of the one-split and two-split tests and their combined tests in Example 5 at a nominal level $\alpha = 0.05$. The data-adaptive tuning scheme is applied.}
    \centering
  \scalebox{.88}{
  \begin{tabular}{@{}cccccccccccccc@{}} \toprule
  & Test & \phantom{a} & $r$  & \phantom{a} & Type \rom{1} error & \phantom{a}& Power(1 - Type II error)  \\
  \midrule
  & One-split && 0.00 && 0.044 && (0.55, 0.98, 0.96) \\
  & && 0.25 && 0.050 && (0.61, 0.99, 1.00) \\
  & && 0.50 && 0.052 && (0.89, 1.00, 1.00) \\
  \midrule
  & Two-split && 0.00 && 0.040 && (0.09, 0.32, 0.35) \\
  & && 0.25 && 0.035 && (0.18, 0.51, 0.58) \\
  & && 0.50 && 0.039 && (0.09, 0.80, 0.79) \\
  \midrule
  & Comb. one-split && 0.00 && 0.029 && (0.64, 1.00, 1.00) \\
  &  &&  0.25 && 0.046 && (0.86, 1.00, 1.00) \\
  &  &&  0.50 && 0.033 && (0.98, 1.00, 1.00) \\
  \midrule
  & Comb. two-split && 0.00 && 0.018 && (0.04, 0.38, 0.31) \\
  &  && 0.25 && 0.030 && (0.10, 0.70, 0.65) \\
  &  && 0.50 && 0.022 && (0.09, 0.95, 0.98) \\
  \bottomrule
  \end{tabular}}
  \label{tab:sim_cor}
  \end{table}

  \begin{table*}[!h]\centering
    \caption{Empirical Type \rom{1} errors and powers of the different combined methods for the one-split test in \textbf{Example 6} at a nominal level $\alpha = 0.05$.}
    \label{tab:sim_cp}
    \scalebox{1.0}{
    \begin{tabular}{@{}cccccccccccccc@{}} \toprule
    & \phantom{a} & Test & \phantom{a} & $B$ & \phantom{a} & $(L, d)$ & \phantom{a} &  Comb. method  & \phantom{a} & Type \rom{1} error & \phantom{a}& Power(1 - Type II error) & \phantom{a}  \\
    \midrule
    && Comb. one-split && 0.20 && (3, 128) && Hommel && 0.019 && (0.27, 0.93, 0.93) \\
    &&  &&  && && Bonferroni && 0.044 && (0.43, 0.95, 0.98) \\
    &&  &&  && && 1$^{\text{st}}$-Quantile && 0.004 && (0.13, 0.89, 0.95) \\
    &&  &&  && && median && 0.000 && (0.02, 0.69, 0.75) \\
    &&  &&  && && Cauchy && 0.050 && (0.41, 1.00, 1.00) \\
    &&  &&  && && harmonic && 0.014 && (0.20, 0.84, 0.94) \\
    \midrule
    && Comb. one-split && 0.40 && (4, 32) && Hommel && 0.054 && (1.00, 1.00, 1.00) \\
    &&  &&  && && Bonferroni && 0.097 && (1.00, 1.00, 1.00) \\
    &&  &&  && && 1$^{\text{st}}$-Quantile && 0.011 && (1.00, 1.00, 1.00) \\
    &&  &&  && && median && 0.000 && (1.00, 1.00, 1.00) \\ 
    &&  &&  && && Cauchy && 0.099 && (1.00, 1.00, 1.00) \\
    &&  &&  && && harmonic && 0.035 && (1.00, 1.00, 1.00) \\
    % && Comb. two-split && 6000 && 0.00 && 0.005 &&  \\
    \bottomrule
    \end{tabular}}
    \end{table*}

\subsection{Comparison with the likelihood ratio test for a non-blackbox learner}
{This subsection compares the proposed tests with the likelihood ratio test (LRT) for a logistic regression, although 
the former is designed for
a blackbox learner. In simulations, we generate a random sample $(\bm X_i, Y_i)_{i=1}^N$ as follows. First, we generate a feature vector $\bm{X}$ and the regression parameter vector $\bm{\theta}$ from $N(\bm{0}, \bm{I}_d)$. Second, we generate a binary response $Y$ as
$Y = \sign( \bm{\theta}^\intercal \bm{Z} + .1 \epsilon)$ with $\bm{Z}_{1:10} = \bm{0}$ and $\bm{Z}_{11:100} = \bm{X}_{11:100}$.
Now consider a hypothesis test in Section 2 to determine if $\bm{X}_\mathcal{S}$ is functionally relevant to
the prediction of $\bm Y$, consider null $H_0$ and alternative $H_a$ hypotheses in three cases: (i) $\mathcal{S}=\{1, \cdots, 10 \}$, (ii) $\mathcal{S} = \{ 5, \cdots, 15 \}$, (iii) $\mathcal{S} = \{ 10, \cdots, 15 \}$,
where the sample size $N$ is $500, 800, 1000$ and $d=100$.}

% $H_0: R(f^*) - R_\mathcal{S}(g^*) = 0$ versus $H_a: R(f^*) - R_\mathcal{S}(g^*) < 0$. 
%We examine three index sets of hypothesized features $\mathcal{S}$: (i) $\mathcal{S}=\{1, \cdots, 10 \}$, (ii) $\mathcal{S} = \{ 5, \cdots, 15 \}$, (iii) $\mathcal{S} = \{ 10, \cdots, 15 \}$, with the sample size $N=500, 800, 1000$ and $d=100$.} 

{For implementation, we fit a logistic regression model with sample $(\bm{X}_i, Y_i)_{i=1}^N$ via stochastic gradient descent with a learning rate 0.05 for LRT based on the Github repo\footnote{{https://gist.github.com/rnowling/ec9c9038e492d55ffae2ae257aa4acd9}}. For the proposed tests, we use the same fitting and splitting parameters for data-adaptive scheme as in Section 6.2.}

\begin{table}[!ht]\centering
  \caption{{Empirical Type \rom{1} errors and powers of the likelihood ratio test, the one-split and two-split tests, and their 
combined tests at a nominal level $\alpha = 0.05$. The likelihood ratio uses the asymptotic $\chi$-square distribution for the null
distribution.}}
\label{tab:sim_linear}
\scalebox{.8}{
\begin{tabular}{@{}cccccccccccccc@{}} \toprule
 & Test & \phantom{a} & sample size  & \phantom{a} & Type \rom{1} error & \phantom{a}& Power(1 - Type II error) \\
\midrule
& One-split && 500 && 0.040 && (0.15, 0.20) \\
& && 800 && 0.020 && (0.42, 0.44) \\
& && 1000 && 0.040 && (0.69, 0.77) \\
\midrule
& Two-split && 500 && 0.032 && (0.13, 0.13) \\
& && 800 && 0.030 && (0.18, 0.18) \\
& && 1000 && 0.020 && (0.39, 0.34) \\
\midrule
& Comb. one-split && 500 && 0.042 && (0.19, 0.24) \\
& && 800 && 0.010 && (0.53, 0.59) \\
& && 1000 && 0.019 && (0.79, 0.85) \\
\midrule
& Comb. two-split && 500 && 0.020 && (0.06, 0.15) \\
& && 800 && 0.012 && (0.32, 0.37) \\
& && 1000 && 0.002 && (0.51, 0.50) \\
\midrule
& LRT && 500 && 0.003 && (0.52, 0.55) \\
& && 800 && 0.000 && (0.92, 0.93) \\
& && 1000 && 0.035 && (0.98, 0.99) \\
\bottomrule
\end{tabular}}
\end{table}

% CASE 0: Type 1 error: 0.010
% CASE 1: Power: 0.320
% CASE 2: Power: 0.370

{As indicated in Table \ref{tab:sim_linear}, LRT and the proposed tests 
control the Type \rom{1} error but the proposed tests exhibit a fair yet insubstantial amount of power loss.  The loss 
of power of the proposed test is primarily due to their smaller inference sample. }

\subsection{Inflated Type \rom{1} errors for holdout permutation test (HPT) and permutation test (PT)}

{This subsection demonstrates that HPT and PT can incur inflated Type \rom{1} errors. Algorithm 2 summarizes the procedure for the permutation test.

\begin{algorithm}
    \SetKwInOut{Input}{Input}
    \SetKwInOut{Output}{Output}
    % \underline{function PermT}\;
    \Input{Data $\mathcal{D} = (\bm{x}_i, \bm{y}_i)_{i=1}^N$; Set of hypothesized features: $\mathcal{S}$; Number of permutations $T$}
    \Output{$p$-values for marginal independence}
    Compute the cross-validation score $s_0$ on data $\mathcal{D}$. \\
    \For{$t = 1, \cdots, T$}
      {
      Generate $\mathcal{D}_t$ by simultaneously permuting values of hypothesized features in $H_0$. \\
      Compute the cross-validation score $s_t$ based on data $\mathcal{D}_t$
      }
    Compute $p$-value:
    $$
    \widehat{p} = \frac{\big|\{ s_t \leq s_0 | t = 1, \cdots, T \}\big| + 1}{T + 1}.
    $$
    \caption{Permutation test for feature relevance to prediction.}
    \label{algo:PermT}
\end{algorithm}

Specifically, we consider the same simulation setting in Section 4.2, with $N=2000$, $B=0.1$, $r=0.85$, $p=100$, $\tau=2$, $L=2$, $\varpi = 128$, and $|\mathcal{S}_0| = 3$. The Type \rom{1} errors of the null hypothesis based on $\mathcal{S}=\{1,2,3\}$ for all tests are reported in Table \ref{tab:perm} over 100 simulations. As indicated in Table \ref{tab:perm}, the one-split/two-split tests and their combined tests control Type \rom{1} error, yet neither HPT nor PT could control the Type \rom{1} error under a nominal level.}

\begin{table*}[!ht]\centering
  \caption{{Type \rom{1} errors of the holdout permutation test (HPT), the permutation test (PT), the one-split and two-split tests and their combined tests at a nominal level $\alpha = 0.05$.}}
\label{tab:perm}
\scalebox{1.0}{
\begin{tabular}{@{}cccccccccccccccccc@{}} \toprule \phantom{a} & One-split & \phantom{a} & Two-split & \phantom{a}& Comb. one-split & \phantom{a} & Comb. two-split & \phantom{a} & HPT & \phantom{a} & PT \\
\midrule
& 0.03 && 0.04 && 0.01 && 0.01 && 0.12 && 0.97 & \\
\bottomrule
\end{tabular}}
\end{table*}

\subsection{Effect of size of grids of data-adaptive splitting scheme}
{This subsection demonstrates the effect of size of grids of the perturbation size $\rho$ and the splitting ratio $\zeta$ for the heuristic data-adaptive scheme in Section 5.2.}

{For illustration, we consider the same simulation setting as in Example 1 with $N=6000$, then the grids $\bm{\zeta} = \{ .2, .6 \}, \{.2, .4, .6, .8 \}, \{.2, .3, \cdots, .9\}$, and $\bm{\rho} = \{ .01, .1, 1 \}, \{ .01, .05, .1, .5, 1 \}$ are examined. The Type \rom{1} error and power functions for the proposed methods are summarized in Table \ref{tab:sim_grid}.}

\begin{table*}[!ht]\centering
  \caption{{Empirical Type \rom{1} errors and powers of the one-split and two-split tests with different size of grids at a nominal level $\alpha = 0.05$.}}
\label{tab:sim_grid}
\scalebox{1.0}{
\begin{tabular}{@{}cccccccccccccc@{}} \toprule
& \phantom{a} & Test & \phantom{a} & $\bm{\zeta}$ & \phantom{a} & $\bm{\rho}$ & \phantom{a} & Type \rom{1} error & \phantom{a}& Power(1 - Type II error) & \phantom{a} & Time (Second) & \phantom{a} \\
\midrule
&& One-split && \{.2, .6\} && \{.01, .1, 1\} && 0.020 && (0.65, 1.00, 1.00) && 31.4(1.2) \\
&& &&  && \{.01, .05, .1, .5, 1\} && 0.022 && (0.58, 1.00, 1.00) && 30.4(1.1)\\
\cmidrule{5-8}
&& && \{.2, .4, .6, .8\} && \{.01, .1, 1\} && 0.010 && (0.62, 1.00, 1.00) && 29.4(0.5) \\
&& &&  && \{.01, .05, .1, .5, 1\} && 0.050 && (0.61, 0.99, 1.00) && 41.2(0.3) \\
\cmidrule{5-8}
&& && \{.2, .3, $\cdots$, .9\} && \{.01, .1, 1\} && 0.009 && (0.63, 1.00, 1.00) && 32.2(2.0) \\
&& &&  && \{.01, .05, .1, .5, 1\} && 0.021 && (0.70, 1.00, 1.00) && 32.1(1.2) \\
\midrule
&& Two-split && \{.2, .6\} && -- && 0.032 && (0.17, 0.49, 0.56) && 30.6(0.6) \\
&& && \{.2, .4, .6, .8\} && -- && 0.035 && (0.18, 0.51, 0.58) && 37.0(0.2) \\
&& && \{.2, .3, $\cdots$, .9\} && -- && 0.031 && (0.16, 0.58, 0.62) && 30.3(0.7) \\
\bottomrule
\end{tabular}}
\end{table*}

As indicated in Table \ref{tab:sim_grid}, Type \rom{1} error, power and computation time based on data adaptive splitting method do not significantly affected by the grid sets of $(\zeta, \rho)$ due to the early stopping mechanism.

\subsection{Simulation for model misspecification}
\label{sec:sim_misspec}
{
This subsection examines performance for the proposed tests in situation that the true regression function $f^*$ belongs to a bigger class than a neural network class $\mathcal{H}$. Toward this end, we simulate random samples $(\bm{X}_i, Y_i)_{i=1}^N$ as follows. First, we simulate $\bm{X}_i$ from $N(\bm{0}, \bm{I}_d)$ with $d = 10$. Second, we generate $Y_i$:
$$Y_i = 0.1 X_{i6} + 0.2 X^2_{i7} + 0.3 X^3_{i8} + 0.4 X_{i9} X_{i10} + 0.3 \epsilon,$$ 
where $\epsilon \sim N(0,1)$. Now consider the null hypothesis in (1) to determine if $\bm{X}_\mathcal{S}$ is functionally relevant to the prediction of $Y$ with the true null $H_0$ and alternative $H_a$ hypotheses in three cases: 
(i) $\mathcal{S} = \{1, \cdots, 5\}$, (ii) $\mathcal{S} = \{3, \cdots, 7\}$, (iii) $\mathcal{S} = \{6, 7, 8\}$, where the sample size $N$ is 1000, 2000, 6000. Note that (i) is for Type \rom{1} error analysis and (ii)-(iv) are for power analysis.
}

{As indicated in Table \ref{tab:sim_misspecified}, the proposed tests control the Type \rom{1} errors for all different sample sizes, and the power increases as the sample size becoming larger. The numerical results also confirm the theoretical analysis in Section \ref{sec:example}.}

\begin{table}[!ht]\centering
  \caption{Empirical Type \rom{1} errors and powers of the one-split, two-split tests, and their combined tests in the misspecified situation at a nominal level $\alpha = 0.05$. The data-adaptive scheme is applied to determine the splitting ratio and perturbation size.}
\label{tab:sim_misspecified}
\scalebox{.8}{
\begin{tabular}{@{}cccccccccccccccc@{}} 
\toprule
& Test & \phantom{a} & Sample size & \phantom{a} & Type \rom{1} error & \phantom{a} & Power(1 - Type II error) \\
\midrule
& One-split && 1000 && 0.000 && (0.11, 1.00)  \\
&  && 2000 && 0.000 && (0.56, 1.00)   \\
&  &&  6000 && 0.002 && (0.97, 1.00)  \\
\midrule
& Two-split && 1000 && 0.000 && (0.02, 0.77)  \\
&& & 2000 && 0.001 && (0.33, 0.95)  \\ 
&& & 6000 && 0.001 && (0.94, 1.00)  \\
\midrule
& Comb. one-split && 1000 && 0.028 && (0.15, 1.00) \\
& && 2000 && 0.000 && (0.79, 1.00)  \\
& && 6000 && 0.001 && (1.00, 1.00)  \\
\midrule
& Comb. two-split && 1000 && 0.000 && (0.02, 0.82) \\
& && 2000  &&  0.002 && (0.33, 1.00)  \\
& && 6000  &&  0.002 && (1.00, 1.00)  \\
\bottomrule
\end{tabular}}
\end{table}

\section{Theoretical example}
\label{sec:example}
This section provides a specific theoretical example to illustrate the one-split test, and verify Assumptions A-C. Consider nonparametric regression,
\begin{equation}
\label{eqn:network_example}
Y = f^*(\bm{X})+ \epsilon, \quad \epsilon \sim N(0, \varsigma^2),
\end{equation}
where $f^*(\bm x)$ is an unknown function on $\bm{x} \in [-1,1]^d$. It is known that $f^*(\bm{x})=g^*(\bm z)$ only depends on a subset of features of $\bm x$, in which $\bm{z}_{\mathcal{S}_0}=\bm{0}$ and $\bm{z}_{\mathcal{S}^c_0} = \bm{x}_{\mathcal{S}^c_0}$ with $\mathcal{S}_0 = \{ 1, \cdots, |\mathcal{S}_0| \}$. Given a hypothesized index set $\mathcal{S}$, our goal is to test if $\bm{X}_{\mathcal{S}}$ is relevant to predicting the outcome $Y$, as specified in Section 2.

For illustration, consider $f^*(\bm{x}) = A \big( (\bm{W}^{L})^* A \big( (\bm{W}^{L-1})^* \cdots A((\bm{W}^{1})^* \bm{x}) \big) \big)$, where $A(\cdot)$ is the ReLU activation function, $(\bm{W}^{l})^* = ((w^{l}_{ij})^*) \in \mathbb{R}^{d_{l} \times d_{l-1}}$ is a weight matrix, $\| (\bm{w}_j^{l})^* \|_2 = \tau/d_{l-1}^{1/2}$, $(\bm{w}_j^{l})^*$ is the $j$-th column of the matrix $(\bm{W}^l)^*$, $\tau > 0$ is a constant, $d_l$ is the width for the $l$-th layer, and $d_0 = d, \ d_L = 1, \ d_1 = \cdots = d_{L-1} = \varpi$ and $L$ is the depth of the network. Clearly, $f^* \in \mathcal H$, where $\mathcal{H}$ is defined as:
\begin{align*}
& \mathcal{H} = \{ f(\bm x)=A \big( \bm{W}^{L} A \big(\bm{W}^{L-1} \cdots A(\bm{W}^{1} \bm{x}) \big) \big): \\
& \hspace{4cm} \|\bm{W}^{l}\|_2 \leq \tau, \| \bm{W}^{l} \|_{2,1} \leq \tau \}.
\end{align*}

Given an estimation sample $(\bm{X}_i, Y_i)_{i=1}^n$ and an inference sample $(\bm{X}_j, Y_{j})_{j=n+1}^{n+m}$, consider a loss function $l(\hat{y}, y) = (\hat{y} - y)^2$, where $\hat{y}$ is the predicted outcome of $y$ and the prediction functions $(\widehat{f}_n, \widehat{g}_n)$ are obtained:
\begin{align}
\label{eqn:empirical_min}
& \widehat{f}_n = \argmin_{f \in \mathcal{H}} \ n^{-1} \sum_{i=1}^n l\big(f(\bm{X}_i), Y_i \big); \nonumber \\
& \widehat{g}_n = \argmin_{g \in \mathcal{H}} \ n^{-1} \sum_{i=1}^n l\big(g(\bm{Z}_i), Y_i \big).
\end{align}

To solve \eqref{eqn:empirical_min}, we apply a stochastic gradient descent (SGD) algorithm. In general, SGD finds a local minimum of a nonconvex objective function \cite{ge2015escaping} but a global minimizer in some special situations \cite{raginsky2017non,wu2018sgd}.

Lemma \ref{lem:example} is a version of Theorems 2 and 4, leading to the desired asymptotic null distribution and power of the one-split test in this specific example.

\begin{lemma}
\label{lem:example} If $m = o(n^{2\gamma})$ with $\gamma = 1-\omega$ for any $\omega > 0$, then the one-split test based on $\widehat{f}_n$ and $\widehat{g}_n$ from \eqref{eqn:empirical_min} satisfies: under $H_0$,
\begin{align*}
& \lim_{n \to \infty} \mathbb{P} \big(P^{(1)} \leq \alpha | H_0 \big) = \alpha, \quad \lim_{n \to \infty} \mathbb{P} \big(\bar{P}^{(1)} \leq \alpha | H_0 \big) \leq \alpha.
\end{align*}
Under $H_a$,
\begin{align*}
& \lim_{\delta \to \infty} \lim_{n \to \infty} \sup \beta_n(\delta)= 0, \hspace{.8cm}  \lim_{\delta \to \infty} \lim_{n \to \infty} \sup \bar{\beta}_n(\delta)= 0.
\end{align*}
\end{lemma}

As a remark, we note that Lemma \ref{lem:example} can be extended to a misspecified model situation, where $f^* \notin \mathcal{H}$ but belongs to a larger space such as $\mathcal{C}_d^{\xi}$, the $\xi$-H\"older functional space. 
In such a situation, the approximation error of $f^*$ by $\mathcal{H}$ plays a role in the rate of convergence. Still, the rate in Assumption A can be obtained; for instance, the rate is $n^{-\xi / (2\xi + d + 5)}$ for a neural net with one hidden layer \cite{mccaffrey1994convergence}, and the rate is $n^{-2\xi/(2\xi + d)} (\log n)$ for a two-layer neural net with the sigmoid activation function \cite{kohler2005adaptive,kohler2016nonparametric}. Moreover, the numerical experiment for a misspecified model situation is illustrated in Section \ref{sec:sim_misspec}.

\section{Technical proofs}

In this section, we rewrite $m$ as $m_n$ to emphasize the monotonicity of $m$ as a subsequence of $n$, that is, $m_1 < \cdots < m_n$.

\noindent \textbf{Proof of Lemma 1.} We first prove that $\bm{Y} \perp \bm{X}_\mathcal{S} \mid \bm{X}_{\mathcal{S}^c}$ yields $ R(f^*) - R_{\mathcal{S}}(g^*) = 0$. To find $f^*$ and $g^*$, it suffices to consider the pointwise minimization of $R(f)$ and $R_{\mathcal{S}}(g)$, that is, for any $\bm{x}$, we have
\begin{align*}
f^*(\bm{x}) & = \argmin_{u} \mathbb{E}\big( l( u, \bm{Y}) | \bm{X}_{\mathcal{S}} = \bm{x}_{\mathcal{S}}, \bm{X}_{\mathcal{S}^c} = \bm{x}_{\mathcal{S}^c} \big) \\ 
& = \argmin_{u} \mathbb{E}\big( l( u, \bm{Y}) | \bm{X}_{\mathcal{S}^c} = \bm{x}_{\mathcal{S}^c} \big) \\
& = \argmin_{u} \mathbb{E}\big( l( u, \bm{Y}) | \bm{Z}(\bm{X}) = \bm{z}(\bm{x}) \big) = g^*(\bm{z}(\bm{x})),
\end{align*}
where the second equality follows from the conditional independence. Therefore, $R(f^*) = \mathbb{E}\big( l( f^*(\bm{X}), \bm{Y} ) \big) = \mathbb{E} \big( l( g^*(\bm{Z}(\bm{X})), \bm{Y} ) \big) = R_{\mathcal{S}}(g^*)$.

Next, we show that $H_0$ is equivalent to conditional independence almost surely, if the cross-entropy loss $l(f(\bm{X}), Y) = - \bm{1}_{Y}^\intercal \log( f(\bm{X}) )$ is used in Section 2. Note that $\bm{f}_{k}^*(\bm{x}) = \mathbb{P}(Y=k| \bm{X}=\bm{x})$ and $\bm{g}_{k}^*(\bm{z}) = \mathbb{P}(Y=k| \bm{Z}(\bm{X})=\bm{z}(\bm{x}))$, we have
\begin{align*}
0 & = R(f^*) - R_{\mathcal{S}}(g^*) = \mathbb{E}\Big( \bm{1}^\intercal_Y \log\big( \frac{\bm{f}^*(\bm{X})}{\bm{g}^*(\bm{Z}(\bm{X}))}\big) \Big) \\
& = \mathbb{E} \Big( \text{KL} \big(\bm{f}^*(\bm{X}), \bm{g}^*(\bm{Z}(\bm{X})) \big) \Big),
\end{align*}
which yields that $\text{KL} \big(\bm{f}^*(\bm{X}),  \bm{g}^*(\bm{Z}(\bm{X})) \big) = 0$ with probability one, and $\text{KL}(\cdot, \cdot)$ is the Kullback–Leibler divergence. Thus, $\bm{f}^*(\bm{X}) = \bm{g}^*(\bm{Z}(\bm{X}))$ with probability one. This leads to the desirable results. \EOP

\noindent \textbf{Proof of Theorems 1 and Theorem \ref{thm:type1}.} 
Note that $\Lambda_n^{(l)}= T^{(l)}_{n,1} + T^{(l)}_{n,2} + T^{(l)}_{n,3}$, where $T^{(l)}_{n,1}$, $T^{(l)}_{n,2}$, and $T^{(l)}_{n,3}$ are defined as 
\begin{align}
& T^{(l)}_{n,1} = \frac{(m^{(l)}_n)^{1/2}}{\widehat{\sigma}^{(l)}_n} \Big( \frac{1}{m^{(l)}_n} \sum_{j=1}^{m^{(l)}_n} \big( \Delta^{(l)}_{n,j} - \mathbb{E}( \Delta^{(l)}_{n,j} | \mathcal{E}_n ) \big) \Big), \nonumber \\
& T^{(l)}_{n,2} = \frac{(m^{(l)}_n)^{1/2}}{\widehat{\sigma}^{(l)}_n}\Big( R(\widehat{f}_n) - R(f^*) - \big( R_\mathcal{S}(\widehat{g}_n) - R_\mathcal{S}(g^*) \big) \Big), \nonumber \\
& T^{(l)}_{n,3} = \frac{(m^{(l)}_n)^{1/2}}{\widehat{\sigma}^{(l)}_{n}} \big( R(f^*) - R_\mathcal{S}(g^*) \big), \nonumber
\end{align}
where $m_n^{(l)} = m_n$ if $l=1$ and $m_n^{(l)} = m_n/2$ if $l=2$, and $T^{(1)}_{n,3} = T^{(2)}_{n,3} = 0$ under $H_0$. 

Now consider $T^{(l)}_{n,1}$ and $T^{(l)}_{n,2}$ separately. To proceed, we first show that $\widehat{\sigma}_n^{(1)} \stackrel{p}{\longrightarrow} \sigma^{(1)}$ and $\widehat{\sigma}_n^{(2)} \stackrel{p}{\longrightarrow} \sigma^{(2)}$. Specifically, for $l = 1, 2$,
\begin{align*}
& (\widehat{\sigma}^{(l)}_{n})^2 = \frac{m^{(l)}_n}{m^{(l)}_n - 1} \Big( \frac{1}{m_n^{(l)}} \sum_{j=1}^{m^{(l)}_n} (\Delta^{(l)}_{n,j})^2 - \big( \frac{1}{m_n^{(l)}} \sum_{j=1}^{m^{(l)}_n} \Delta^{(l)}_{n,j} \big)^2 \Big) \\
& = \frac{m^{(l)}_n}{m^{(l)}_n - 1} \Big( \frac{1}{m_n^{(l)}} \sum_{j=1}^{m^{(l)}_n} \big( (\Delta^{(l)}_{n,j})^2 - \mathbb{E}\big( (\Delta^{(l)}_{n,j})^2 | \mathcal{E}_n \big) \big)  \Big) \\
& \quad + \frac{m^{(l)}_n}{m^{(l)}_n - 1} \Big( \big(\frac{1}{m_n^{(l)}} \sum_{j=1}^{m^{(l)}_n} ( \mathbb{E}(\Delta^{(l)}_{n,j}|\mathcal{E}_n) - \Delta^{(l)}_{n,j} ) \big)  \\
& \hspace{3.5cm} \big(\frac{1}{m_n^{(l)}} \sum_{j=1}^{m^{(l)}_n} ( \mathbb{E}(\Delta^{(l)}_{n,j}|\mathcal{E}_n) + \Delta^{(l)}_{n,j} ) \big) \Big) \\
& \quad + \frac{m^{(l)}_n}{m^{(l)}_n - 1} \Big( \Var( \Delta^{(l)}_n | \mathcal{E}_n ) \Big) \stackrel{p}{\longrightarrow} (\sigma^{(l)})^2 , 
\end{align*}
which follows from the continuous mapping theorem, Assumption C 
for the one-split test or Assumption C$'$ for the two-split test, and 
the fact that
\begin{align*}
	& \frac{1}{m^{(l)}_n} \sum_{j=1}^{m^{(l)}_n} \big(\Delta^{(l)}_{n,j} - \mathbb{E}( \Delta^{(l)}_{n,j} |\mathcal{E}_n) \big) \stackrel{p}{\longrightarrow} 0, \\ 
	& \frac{1}{m^{(l)}_n} \sum_{j=1}^{m^{(l)}_n} \big( (\Delta^{(l)}_{n,j})^2 - \mathbb{E}( (\Delta^{(l)}_{n,j})^2 | \mathcal{E}_n) \big) \stackrel{p}{\longrightarrow} 0,
\end{align*}
which are obtained from the law of large number of the triangular array $\{ \Delta^{(l)}_{n,j} \}_{1 \leq j \leq m_n}$ and Assumptions B and B$'$, c.f., Corollary 9.5.6 of \cite{cappe2006inference}.

Consequently, when $m = o(n^{2\gamma})$, it follows from Assumption A and $\widehat{\sigma}^{(l)}_n \stackrel{p}{\longrightarrow} \sigma^{(l)} > 0$ that 
$$
T^{(l)}_{n,2} = \frac{\sqrt{m_n}}{\widehat{\sigma}^{(l)}_n}\Big( R(\widehat{f}_n) - R(f^*) - \big( R_\mathcal{S}(\widehat{g}_n) - R_\mathcal{S}(g^*) \big) \Big) \stackrel{p}{\longrightarrow} 0.
$$
Moreover, 
\begin{align}
T^{(l)}_{n,1} & = \frac{\sigma^{(l)}}{\widehat{\sigma}_n^{(l)}} \frac{1}{(m^{(l)}_n)^{1/2}  \sigma^{(l)}} \Big( \sum_{j=1}^{m^{(l)}_n} \big( \Delta^{(l)}_{n,j} - \mathbb{E}(\Delta^{(l)}_{n,j} | \mathcal{E}_n ) \big) \Big) \nonumber \\
& \stackrel{d}{\longrightarrow} N(0,1),
\end{align}
which follows from the continuous mapping theorem, Slutsky’s Lemma, and the central limit Theorem of the triangular array $\{ \Delta^{(l)}_{n,j} \}_{1\leq j \leq m_n}$, and Assumptions B or B$'$, c.f., Corollary 9.5.11 of \cite{cappe2006inference}. The desired result then follows. This completes the proof. \EOP

\noindent \textbf{Proof of Theorems 2 and \ref{thm:TS_subsamples_type1}.} For $q$-order combined tests, 
let $A = \big \{ \bar{P}^{(l)} \leq \alpha \big \}$ and $B = \big\{ \sum_{u=1}^U \mathbb{I}( P_{u}^{(l)} \leq \frac{q \alpha}{U}) \geq q \big\}$. Since $A=\big \{ P_{(q)}^{(l)} \leq  \frac{q \alpha}{U} \big \}= B$, by Markov's inequality, it follows from the assumptions that either Theorem 1 or Theorem \ref{thm:type1} holds.
Hence,
\begin{align*}
\mathbb{P}(A|H_0) & = \mathbb{P}(B|H_0) \leq \frac{\sum_{u=1}^U \mathbb{P}\big( P^{(l)}_u \leq \frac{q \alpha}{U} | H_0 \big)}{q} \\
& \to \frac{U \mathbb{P}\big( \Phi(Z) \leq \frac{q \alpha}{U}  \big)}{q} = \alpha, \text{ as $n \to \infty$,}
\end{align*}
where $Z$ follows $N(0,1)$, $\Phi(Z)$ follows the uniform distribution on $[0,1]$,  and the last equality follows from continuous mapping theorem. 

For Hommel combined test, according to the proof of 3.3 in \cite{hommel1983tests}, when $n \to \infty$, we have 
\begin{align*}
\mathbb{P} \big( \bar{P}^{(l)} \leq \alpha | H_0 \big) & \leq \sum_{i=1}^{U-1} \frac{1}{i(i+1)} \sum_{u=1}^U \mathbb{P}\big( P_u^{(l)} \leq \frac{\alpha i }{C_U U} | H_0 \big) \nonumber \\
& + \frac{1}{U} \sum_{u=1}^U \big( P_u^{(l)} \leq \frac{\alpha}{C_U} | H_0 \big) \to \alpha. 
\end{align*}
This completes the proof. \EOP

\noindent \textbf{Proof of Theorems 3.1 and \ref{thm:TS_power}.} Let $\delta^{(1)} =  \delta $ and $\delta^{(2)} = \delta/ \sqrt{2}$, using the same argument in the proof of Theorems 1 and \ref{thm:type1}, we have that $T^{(l)}_{n,2} \stackrel{p}{\longrightarrow} 0$ when $m = o(n^{2\gamma})$, and $T^{(l)}_{n,1}\stackrel{d}{\longrightarrow} N(0,1)$. 
Note that $T^{(l)}_{n,3} = \frac{\sqrt{m^{(l)}_n}}{\widehat{\sigma}^{(l)}_{n}} \big( R(f^*) - R_\mathcal{S}(g^*) \big) = - \delta^{(l)} / \widehat{\sigma}_n^{(l)}$. By Slutsky's theorem, we have
\begin{equation}
\label{pf:power_dis}
\Lambda^{(1)}_n \stackrel{d}{\longrightarrow} N(- \delta^{(1)} / \sigma^{(1)}, 1), \quad \Lambda^{(2)}_n \stackrel{d}{\longrightarrow} N(- \delta^{(2)} / \sigma^{(2)}, 1).
\end{equation}
Consequently, denote $\beta^{(1)}_n(\delta) = \beta_n(\delta)$, we have
$$
\lim_{n \to \infty} \inf \beta_n^{(l)}(\delta)= \Phi\big( z_\alpha - \frac{\delta^{(l)}}{\sigma^{(l)}}  \big); \quad l=1,2.
$$
The desired result then follows. This completes the proof. \EOP

\noindent \textbf{Proof of Theorems 3.2 and \ref{thm:TS_cp_power}.} Denote $\delta^{(1)} =\delta $ and $\delta^{(2)} = \delta/ \sqrt{2} $. We first prove for $q$-order combined tests.
Note that $\bar{\pi}_n^{(l)}(\delta) = 1 - \bar{\beta}^{(l)}_n(\delta)$. By Markov's inequality, Type \rom{2} error is upper bounded by $\mathbb{P}\big( \bar{P}^{(l)} \geq \alpha | H_a \big) \leq \min\Big(\frac{U}{\alpha q} \mathbb{E} \big( P_{(q)}^{(l)} | H_a \big),1\Big)$. To bound the expectation of an order statistic based on dependent samples, we apply (1) of \cite{bertsimas2006tight}, which is a version of \cite{arnold1979bounds}:
\begin{align}  
\label{inq}
\mathbb{E} \big( P_{(q)}^{(l)} | H_a \big) \leq \bar{\mu}+ \Big(\frac{q - 1}{U-q +1} \sum_{u=1}^U \big(\sigma^2_u+(\mu_u-\bar{\mu})^2\big)\Big)^{1/2}, 
\end{align}
where $\bar{\mu}= U^{-1}\sum_{u=1}^U \mu_u$, $\mu_u=\mathbb{E}(P^{(l)}_u|H_a)$ and $\sigma^2_u=\Var(P^{(l)}_u|H_a)$. 

For $u=1,\cdots,U$, by \eqref{pf:power_dis} and Portmanteau's theorem, $\mathbb{E} \big( P_u^{(l)} | H_a \big)  \to \mathbb{E} \big( \Phi\big( Z - \frac{\delta^{(l)}}{\sigma^{(l)}} \big) \big)$ as $n\rightarrow \infty$. 
By Corollary 1 of \cite{ellison1964two}, $\mathbb{E} \big( \Phi\big( Z - \frac{\delta^{(l)}}{\sigma^{(l)}} \big) \big)= \Phi\big( - \frac{\delta^{(l)}}{\sqrt{2}\sigma^{(l)}} \big)$. Similarly, $\Var \big( P_u^{(l)} | H_a \big)  \to \Var \big( \Phi\big( Z - \frac{\delta^{(l)}}{\sigma^{(l)}} \big) \big)$; $u=1,\cdots,U$; $\Var \big( \Phi\big( Z - \frac{\delta^{(l)}}{\sigma^{(l)}} \big) \big) = \Phi\big( - \frac{\delta^{(l)}}{\sqrt{2} \sigma^{(l)}} \big) - \Phi^{2}\big( - \frac{\delta^{(l)}}{\sqrt{2} \sigma^{(l)}} \big) - 2T(- \frac{\delta^{(l)}}{\sqrt{2} \sigma^{(l)}}, \frac{\sqrt{3}}{3})$, where $T(\cdot, \cdot)$ is Owen's $T$ function \cite{owen1956tables}.

Therefore, by \eqref{inq}, as $n \rightarrow \infty$, 
\begin{align*}
 \mathbb{E} \big( P_u^{(l)} & | H_a \big) \to \mathbb{E} \big( \Phi\big( Z - \frac{\delta^{(l)}}{\sigma^{(l)}} \big) \big) \\
 & \quad + \Big( \frac{q - 1}{U -q +1} \Var\big(\Phi\big( Z - \frac{\delta^{(l)}}{\sigma^{(l)}} \big) \big)\Big)^{1/2} \\
% & \leq \mathbb{E} \big( \Phi\big( Z - \frac{\delta^{(l)}}{\sigma^{(l)}} \big) \big) + \sqrt{\frac{q - 1}{U- q +1}} \Big( \mathbb{E} \big( \Phi\big( Z - \frac{\delta^{(l)}}{\sigma^{(l)}} \big) \big) - \big(\mathbb{E} \big( \Phi\big( Z - \frac{\delta^{(l)}}{\sigma^{(l)}} \big) \big) \big)^2 \Big)^{1/2} \\
& = \Phi\big( - \frac{\delta^{(l)}}{\sqrt{2} \sigma^{(l)}} \big) \\ 
& \quad + \sqrt{\frac{q - 1}{U - q +1}} \Big( \Phi\big( \frac{\delta^{(l)}}{\sqrt{2} \sigma^{(l)}} \big) - \Phi^{2}\big( \frac{\delta^{(l)}}{\sqrt{2} \sigma^{(l)}} \big) \\
& \quad  - 2T(- \frac{\delta^{(l)}}{\sqrt{2} \sigma^{(l)}}, \frac{\sqrt{3}}{3}) \Big)^{1/2}.
\end{align*}
The desired result then follows. Therefore, for Hommel combined test, 
\begin{align*}
\mathbb{P}\big( C_U \min_{1 \leq q \leq U} \frac{U}{q} P_{(q)}^{(l)} \leq \alpha | H_a \big) \geq \max_{1 \leq q \leq U} \mathbb{P}\big( \frac{U}{q} P_{(q)}^{(l)} \leq \frac{\alpha}{C_U} | H_a \big).
\end{align*}
The desired result then follows by taking limits for both sides. This completes the proof. \EOP

\noindent \textbf{Proof of Lemma \ref{lem:example}.} To proceed, let $f_0\in \mathcal{H}$ be a neural network, and its weight matrix is exactly same with that of $g_0$ defined in \eqref{eqn:network_example}, expect that $j$-th $(j \in \mathcal{S}_0)$ column in the first layer is set as zero, which implies that $f^*(\bm{X}) = f_0(\bm{X}) = g_0(\bm{Z}(\bm{X}))$.

To verify Assumption A, it suffices to verify the entropy condition of $\mathcal{H}$. By Theorem I of \cite{guo2019realizing}, for any $\omega > 0$, we have
\begin{align*}
	\log \mathcal{N}\big(u, \mathcal{H}, \| \cdot \|_2 \big) & \leq c(p, \varpi,\tau, L) \log(u^{-1}) = O(u^{-\omega}),
\end{align*}
where $\mathcal{N}\big(u, \mathcal{H}, \| \cdot \|_2 \big)$ is the covering number based on $L_2$-norm, $c(p,\varpi,\tau, L)$ is a constant depends on $p$, $\varpi$, $\tau$, and $L$. By \cite{han2019convergence},
\begin{align}
& R(\widehat{f}_n) - R(f^*) = \mathbb{E}\big( \widehat{f}_n(\bm{X}) - f^*(\bm{X}) \big)^2 = O_p( n^{-1 + \omega}), \nonumber \\
& R_\mathcal{S}(\widehat{g}_n) - R_\mathcal{S}(g^*) = \mathbb{E}\big( \widehat{g}_n(\bm{X}) - g^*(\bm{X}) \big)^2 = O_p( n^{-1 + \omega}).
\end{align}
Therefore, $\gamma = 1 - \omega$ for Assumption A with any $\omega > 0$. Then Assumptions B and B$'$ follow from the fact that $f \in \mathcal{H}$ is upper bounded by a constant, that is
\begin{align}
\label{proof:bdd}
\sup_{\bm{x} \in [-1, 1]^d} & |f(\bm{x})| = \sup_{\bm{x} \in [-1, 1]^d} \big| A \big( \bm{W}^{L} \cdots A (\bm{W}^{1} \bm{x}) \big) \big) \big| \nonumber \\
& \leq \big(\prod_{l=1}^L \| \bm{W}^l \|_2 \big) \sup_{\bm{x} \in [-1, 1]^d} \| \bm{x} \|_2 \leq \sqrt{p} \tau^L,
\end{align}
where the second last inequality follows from the definition of the matrix norm.
Next, we verify Assumptions C and C$'$. Let $\mathbb{E}_n(\cdot) = \mathbb{E}(\cdot|\mathcal{E}_n)$, $\Var_n(\cdot) = \Var(\cdot|\mathcal{E}_n)$, $\Psi(f,g,\bm{U}) = l(f(\bm{X}), Y) -l(g(\bm{Z}(\bm{X})), Y)$, and $\bm{U} = (\bm{X}, Y)$. Then,
\begin{align*}
{\Var}_n ( & \Delta^{(1)}_{n,1} ) = {\Var}_n \big( \Psi(\widehat{f}_n,\widehat{g}_n,\bm{U}) \big) + \rho_n^2 \nonumber \\
& = {\Var}_n \big( \Psi(\widehat{f}_n,f^*,\bm{U}) + \Psi(f^*, g^*,\bm{U}) \\
& \quad + \Psi(g^*, \widehat{g}_n,\bm{U}) \big) + \rho_n^2 \nonumber \\
& = {\Var}_n \big( \Psi(\widehat{f}_n,\widehat{g}_n,\bm{U}) \big) + {\Var}_n \big( \Psi(f^*, g^*,\bm{U}) \big) \\
& \quad  + {\Var}_n \big( \Psi(g^*, \widehat{g}_n,\bm{U}) \big) \\
& \quad + 2\Cov \big( \Psi(\widehat{f}_n,\widehat{g}_n,\bm{U}), \Psi(f^*, g^*,\bm{U}) \big) \\ 
& \quad + 2\Cov \big( \Psi(\widehat{f}_n,\widehat{g}_n,\bm{U}), \Psi(g^*, \widehat{g}_n,\bm{U}) \big) \nonumber \\
& \quad + 2\Cov \big( \Psi(f^*, g^*,\bm{U}), \Psi(g^*, \widehat{g}_n,\bm{U})\big)+ \rho_n^2  \\ 
& \stackrel{p}{\longrightarrow} {\Var} \big( \Psi(f^*, g^*,\bm{U}) \big) + \rho_n^2 = (\sigma^{(1)})^2, \nonumber
\end{align*}
where the last equality follows from the uniform boundedness of $\mathcal{H}$ in \eqref{proof:bdd} and the fact that ${\Var}_n \big( \Psi(g^*,\widehat{g}_n,\bm{U}) \big), {\Var}_n \big( \Psi(\widehat{f}_n,f^*,\bm{U}) \big) \stackrel{p}{\longrightarrow} 0$. Specifically, 
\begin{align*}
{\Var}_n & \big( \Psi(\widehat{f}_n,f^*,\bm{U}) \big) \leq \mathbb{E}_n \big( \Psi^2(\widehat{f}_n,f^*,\bm{U}) \big) \\
& = \mathbb{E}_n \Big( \big( \widehat{f}_n(\bm{X}) - f^*(\bm{X}) \big)^2 \big( \widehat{f}_n(\bm{X}) + f^*(\bm{X}) - 2Y \big)^2  \Big) \nonumber \\
& \leq (2\sqrt{p}\tau + 4 \varsigma^2) \mathbb{E}_n \Big( \big( \widehat{f}_n(\bm{X}) - f^*(\bm{X}) \big)^2 \Big) \\ 
& = (2\sqrt{p}\tau + 4 \varsigma^2) \big( R(\widehat{f}_n) - R({f}^*) \big) \stackrel{p}{\longrightarrow} 0. \nonumber
\end{align*}
Similarly, we can show that ${\Var}_n \big( \Psi(g^*,\widehat{g}_n,\bm{U}) \big) \stackrel{p}{\longrightarrow} 0$.

Moreover, for $\Delta_n^{(2)}$, using the same argument, we have
\begin{align*}
{\Var}_n & \big( \Delta^{(2)}_n \big) = {\Var}_n \big( l(\widehat{f}_n(\bm{X}), Y) -l(\widehat{g}_n(\bm{Z}'), Y') \big) \\
& = {\Var}_n \big( l(\widehat{f}_n(\bm{X}), Y)\big) + {\Var}_n \big(l(\widehat{g}_n(\bm{Z}), Y) \big) \\
& \stackrel{p}{\longrightarrow} \Var( l(f^*(\bm{X}), Y) ) + \Var( l(g^*(\bm{Z}), Y) ) = (\sigma^{(2)})^2.
\end{align*}
The desired result then follows. This completes the proof. \EOP

\noindent \textbf{Proof of Lemma 2.} By the definitions of $n$ and $m$ in Section 3.1, we have 
$$ m = N - n \leq N - x_0 =  N_0 \log(x_0) / 2 / \log(N_0 / 2) = o( n^{2\gamma} ), $$
where $\gamma > 0$ is any fixed constant in Assumption A, and the last equality follows from $n \geq x_0$. This completes the proof. \EOP

% use section* for acknowledgment

% Can use something like this to put references on a page
% by themselves when using endfloat and the captionsoff option.
\ifCLASSOPTIONcaptionsoff
  \newpage
\fi

% trigger a \newpage just before the given reference
% number - used to balance the columns on the last page
% adjust value as needed - may need to be readjusted if
% the document is modified later
%\IEEEtriggeratref{8}
% The "triggered" command can be changed if desired:
%\IEEEtriggercmd{\enlargethispage{-5in}}

% references section

% can use a bibliography generated by BibTeX as a .bbl file
% BibTeX documentation can be easily obtained at:
% http://mirror.ctan.org/biblio/bibtex/contrib/doc/
% The IEEEtran BibTeX style support page is at:
% http://www.michaelshell.org/tex/ieeetran/bibtex/
\bibliographystyle{IEEEtran}
% argument is your BibTeX string definitions and bibliography database(s)
\bibliography{IEEEabrv,inf}
\end{document}
